# Supplementary material for: The Role of Recurrency in Image Segmentation for Noisy and Limited Sample Settings
Source: arXiv:2412.15734 source file (2024-12-20)
Supplement: Supplementary file 1 [file appendix.tex]

\input{appendix/noise/noise}
