# Supplementary material for: The Role of Recurrency in Image Segmentation for Noisy and Limited Sample Settings
Source: arXiv:2412.15734 source file (2024-12-20)
Supplement: Supplementary file 2 [file som.tex]

\subsection{Self-organizing dynamics explain neuron response}

\begin{figure}[ht]
    \centering
    \input{results/som/figures/neuron_response}
    \caption{Neuron response dynamics under the self-organizing algorithm.}
    \label{fig:som_neuron_response}
\end{figure}
