# Supplementary material for: The Role of Recurrency in Image Segmentation for Noisy and Limited Sample Settings
Source: arXiv:2412.15734 source file (2024-12-20)
Supplement: Supplementary file 3 [file neuron_response.tex]

\begin{tikzpicture}

    \node (fig1) at (0,0) {\includegraphics[width=0.45\textwidth]{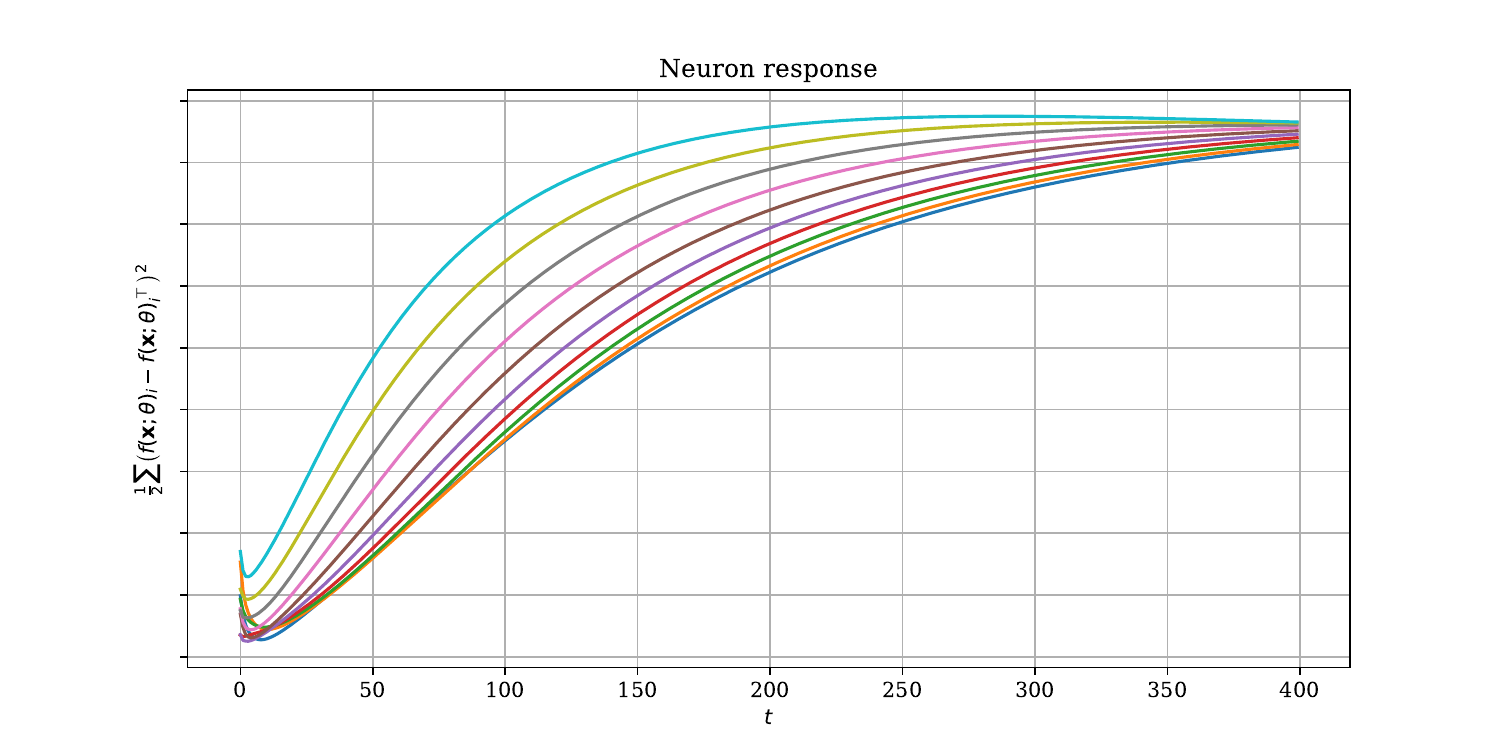}};
    \node (fig2) [anchor=west] at ($(fig1.east)+(0.,0)$) {\includegraphics[width=0.45\textwidth]{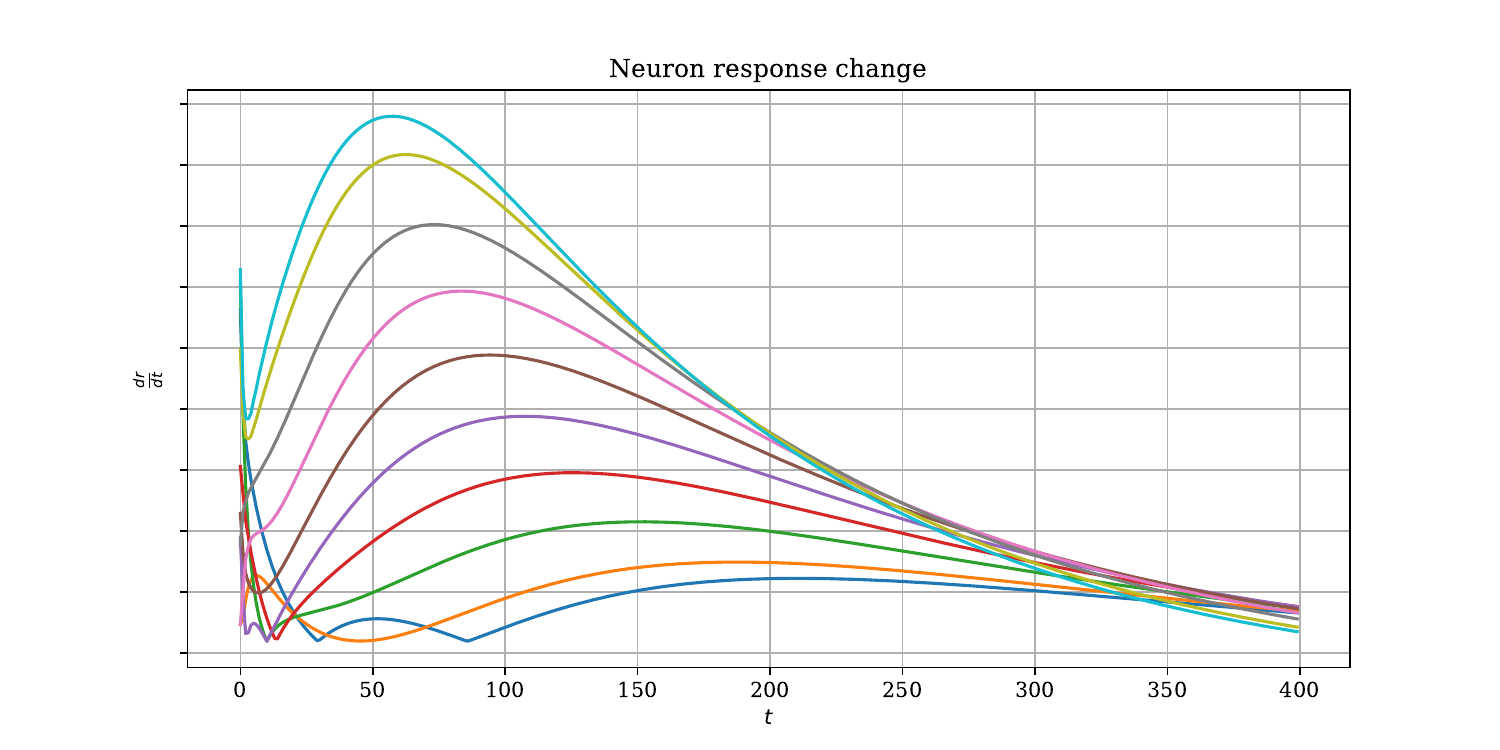}};

    \node (fig1_legend) at ($(fig1.west)+(0.75,2)$) {\large{\textbf{A}}};
    \node (fig2_legend) at ($(fig2.west)+(0.75,2)$) {\large{\textbf{B}}};
\end{tikzpicture}
